# Supplementary material for: Quantum Cognitively Motivated Decision Fusion for Video Sentiment Analysis
Source: arXiv:2101.04406 source file (2021-05-18)
Supplement: Supplementary file 1 [file appendix.tex]

\begin{appendices}

\section{Appendix I: Correlations of Observables}
\label{sec:exp_correlations}

Suppose $M$ be an observable corresponding to one modality:
\begin{equation*}
  M = (+1)[M,+] + (-1)[M,-]
\end{equation*}
where $[M,.]= \ket{M,.}\bra{M,.}$.  If $M$ is treated as random variable, it is
possible to express its expectation as
\begin{equation*}
  \text{E}(M) = \text{tr}(\rho M) = (+1)P_m(+1) + (-1) P_m(-1) 
\end{equation*} 
where $\text{tr}(\rho [M,+]) = P_m(+1)$ and $\text{tr}(\rho [M,-]) =
P_m(-1)$. Note that the variables are still real because the observed values,
which are the eigenvalues of the observables, are real although the operators
are defined over the complex field.

The variance of $M$ can be expressed as
\begin{eqnarray*}
  \text{V}(M)
  &=& (+1-\text{E}(M))^2 P_m(+1)\\ &+& (-1-\text{E}(M))^2 P_m(-1)\\
  % &=& ((+1)^2-2\text{E}(M)+\text{E}(M)^2) P_m(+1) + ((-1)^2+2\text{E}(M)+\text{E}(M)^2) P_m(-1)\\
  % &=& (1-2\text{E}(M)+\text{E}(M)^2) P_m(+1) + (1+2\text{E}(M)+\text{E}(M)^2) P_m(-1)\\
  % &=& (P_m(+1)-2\text{E}(M)P_m(+1)+\text{E}(M)^2P_m(+1) +\\
  % & & (P_m(-1)+2\text{E}(M)P_m(-1)+\text{E}(M)^2 P_m(-1)\\
  % &=& 1-2\text{E}(M)(P_m(+1)-P_m(-1))+\text{E}(M)^2 \\
  % &=& 1-2\text{E}(M)^2+\text{E}(M)^2 \\
  &=& 1-\text{E}(M)^2
\end{eqnarray*}
We can assume that observable expectations are zero without loss of
generality. If they were not zero, it is possible to normalize the observables
and define
\begin{equation*}
  \bar{M} = (+1-\text{E}(M))[M,+] + (-1-\text{E}(M))[M,-1]\ .
\end{equation*}
such that
\begin{equation*}
  \text{E}(\bar{M}) = \text{E}(M-\text{E}(M)) = \text{E}(M) -
  \text{E}(\text{E}(M)) = 0
\end{equation*}
As a consequence, suppose $\bar{M} \equiv M$ without loss of
generality. Therefore, $\text{V}(M) = 1$.

Suppose $A,B$ be two observables corresponding to two modalities.  Both
variables have zero expectation and unit variance.  The covariance between $A,B$
can be expressed as the following complex number:
\begin{equation*}
  \text{Cov}(A,B) = \sum_{i \in \{-1,+1\}} \sum_{j \in \{-1,+1\}} (i -
  \text{E}(A)) (j - \text{E}(B)) P_{a,b}(i,j)
\end{equation*}
where
\begin{equation*}
  P_{a,b}(i,j) = \frac{\text{tr}([A,i]\rho[A,i][B,j])}{\text{tr}([A,i]\rho[A,i])}
\end{equation*}
is the probability that $A$ is measured after the measurement of $B$ according
to L{\"{u}}ders' rule \cite{Luders06}.  The covariance between $A,B$ can be
expressed in the following expanded form since both expectations are zero:
\begin{eqnarray*}
  \text{Cov}(A,B)
  &=& \frac{\text{tr}([A,+1]\rho[A,+1][B,+1])}{\text{tr}([A,+1]\rho[A,+1])} + \\
  & & \frac{\text{tr}([A,+1]\rho[A,+1][B,-1])}{\text{tr}([A,+1]\rho[A,+1])} - \\
  & & \frac{\text{tr}([A,-1]\rho[A,-1][B,+1])}{\text{tr}([A,-1]\rho[A,-1])} - \\
  & & \frac{\text{tr}([A,-1]\rho[A,-1][B,-1])}{\text{tr}([A,-1]\rho[A,-1])}
\end{eqnarray*}
The correlation between two any variables $A,B$ is defined as
\begin{equation*}
  \text{Corr}(A,B) = \frac{\text{Cov}(A,B)}{\sqrt{\text{V}(A)}\sqrt{\text{V}(B)}}
\end{equation*}
that is
\begin{equation*}
  \text{Corr}(A,B) = \text{Cov}(A,B)
\end{equation*}
since $V(M)=1$ for $M \in \{A,B\}$.

Then, consider the correlation between $A,B$ and of the pure state
$\rho = \ket{g}\bra{g}$.  We have that
\begin{eqnarray*}
  P_{a,b}(i,j)
  &=& \frac{\text{tr}([A,i]\rho[A,i][B,j])}{\text{tr}([A,i]\rho[A,i])}\\
  &=& \frac{\text{tr}(\ket{A,i}\bra{A,i}\rho\ket{A,i}\bra{A,i}\ket{B,j}\bra{B,j})}{\text{tr}(\ket{A,i}\bra{A,i}\rho\ket{A,i}\bra{A,i})}\\
 &=& \frac{\braket{B,j|A,i}\braket{A,i|g}\braket{g|A,i}\braket{A,i|B,j}}{\braket{A,i|A,i}\braket{A,i|g}\braket{g|A,i}}\\
 &=& \frac{|\braket{B,j|A,i}|^2|\braket{A,i|g}|^2}{|\braket{A,i|g}|^2}\\
 &=& |\braket{B,j|A,i}|^2
\end{eqnarray*}
It follows that
\begin{eqnarray*}
  \text{Corr}(A,B)
  &=& |\braket{B,+1|A,+1}|^2 + \\
  & & |\braket{B,-1|A,-1}|^2 - \\
  & & |\braket{B,+1|A,-1}|^2 - \\
  & & |\braket{B,-1|A,+1}|^2
\end{eqnarray*}

\section{Appendix II: Statistics of Datasets}
\label{datasets}
\begin{table}[htbp]
\large % text size of table content
\centering % center the table
  \begin{tabular}{lSSS}
    \toprule
      \multicolumn{1}{c}{} &
      \multicolumn{3}{c}{\# Utterances} \\
      \cmidrule(r){2-4}
       Dataset & \textbf{$Train$}  & \textbf{$Validation$}   & \textbf{$Test$}  \\
      \hline
      CMU-MOSI & {1284} & {686} & {229}   \\
      CMU-MOSEI & {16265} & {4643} & {1869}  \\
    \bottomrule
  \end{tabular}
  \caption{Distribution of video utterances per Train, Validation, and Test sets for CMU-MOSI and CMU-MOSEI.} 
  \label{comperativeAnalysis}
\end{table}

\section{Appendix III: Extraction of Features}
\label{features}
Extraction feature processs for different modalities are  as follows:
\begin{itemize}
     \item \textbf{Language:} We converted video transcripts into 300-dimensional pre-trained Glove word embeddings (glove.840B.300d)~\cite{pennington2014glove}. 
     \item \textbf{Visual:} Facet \footnote{\href{https://pair-code.github.io/facets/}{https://pair-code.github.io/facets/}} was used to capture facial muscle movement, including per-frame basic and advanced emotions and facial action units.
     \item \textbf{Acoustic} We used  VOCAREP \cite{degottex2014covarep} to extract low-level acoustic features (e.g., 12 Mel-frequency cepstral coefficients, pitch tracking and voiced/unvoiced segmenting features, glottal source parameters, peak slope parameters, and maxima dispersion quotients).
\end{itemize}     
For MOSI, we extracted visual and acoustic features at a frequency of 15$Hz$ and 12.5 $Hz$ respectively. For MOSEI, we extracted at a frequency of 15 $Hz$ and 20$Hz$. We applied word-level alignment, where visual and acoustic features are averaged across the time interval of each spoken word. All sequences in the word-aligned case had length 50 through zero-pad. For each word the dimension of the feature vector was set to 300 (linguistic), 20 (visual), and 5 (acoustic) for MOSI, and 300 (linguistic), 35 (visual), and 74 (acoustic) for MOSEI.  

\section{Appendix IV: Hyperparameters of Uni-modal Classifiers}
For uni-modal classifiers, the Bi-directional GRUs had 300 neurons, each followed by a dense layer consisting of 100 neurons. A grid search is conducted over a hyperparameter pool. We report the final settings in Table \ref{finetuning}. Each uni-modal classifiers was trained for 50 epochs with Adam as the optimizer on the $L_1$ loss function.

\begin{table}[htbp]
\large % text size of table content
\centering % center the table
\resizebox{\columnwidth}{!}{%
  \begin{tabular}{lSSSSSS}
    \toprule
      \multicolumn{1}{c}{} &
      \multicolumn{3}{c}{CMU-MOSI} &
      \multicolumn{3}{c}{CMU-MOSEI} \\
      \cmidrule(r){2-4} \cmidrule(r){5-7}
       Hyperparameter & {$L$}  & {$V$}   & {$A$}  & {$L$}  & {$V$}   & {$A$} \\
      \hline
      Learning Rate & {0.002}  & {0.002}   & {0.002}  & {0.001}  & {0.002}   & {0.001} \\
      Batch Size & {128}  & {128}   & {128}  & {128}  & {32}   & {32} \\
      Gradient Clipping & {0.8}  & {0.5}   & {0.8}  & {0.3}  & {1}   & {0.5} \\
      Output & {64}  & {32}   & {128}  & {128}  & {64}   & {64} \\
      Output Dropout & {0.15}  & {0.2}   & {0.3}  & {0.3}  & {0.5}   & {0.4} \\
      GRU Dropout & {0.2}  & {0.5}   & {0.1}  & {0.3}  & {0.2}   & {0.5} \\
    \bottomrule
  \end{tabular}}
  \caption{Final settings for training uni-modal classifiers on CMU-MOSI and CMU-MOSEI  } 
  \label{finetuning}
\end{table}

\end{appendices}
